# Supplementary material for: Judgment Sieve: Reducing Uncertainty in Group Judgments through Interventions Targeting Ambiguity versus Disagreement
Source: arXiv:2305.01615 source file (2023-05-02)
Supplement: Supplementary file 1 [file s_appendix.tex]

\appendix

\section{This is the appendix}

Placeholder
